# Supplementary material for: Developing Orbital-Dependent Corrections for the Non-Additive Kinetic Energy in Subsystem Density Functional Theory
Source: arXiv:2409.11914 ancillary file (2025-01-10)
Supplement: Supplementary file 1 [file supplementary_material.pdf]

# – Supporting Information –

## Developing Orbital-Dependent Corrections for the Non-Additive Kinetic Energy in Subsystem Density Functional Theory

Larissa Sophie Eitelhuber and Denis G. Artiukhin[1]

Institut für Chemie und Biochemie, Freie Universität Berlin,

Arnimallee 22, 14195 Berlin, Germany

Date: September 18, 2024

[1]Email: denis.artiukhin@fu-berlin.de

# S1 Deriving Kinetic Energy Corrections

Given a normed space $V$ and a continuous linear operator $\hat{A} : V \to V$, the Neumann series is defined as $\sum_{n=0}^{\infty} \hat{A}^n$, where $\hat{A}^0$ is equal to the identity operator $\hat{I}$ on $V$ [1,2]. In case of convergence of the series, the operator $\hat{I} - \hat{A}$ is invertible and the limit of the series is given by its inverse. Using a matrix representation $\mathbf{A}$ for the linear operator $\hat{A}$, this can be re-formulated as

$$\sum_{n=0}^{\infty} \mathbf{A}^n = (\mathbf{I} - \mathbf{A})^{-1}, \tag{1}$$

where $\mathbf{I}$ is the identity matrix. In this work, the expansion of an inverse molecular orbital (MO) overlap matrix $\mathbf{S}^{-1}$ is of interest so that we choose a matrix representation $\mathbf{A} \coloneqq \mathbf{I} - \mathbf{S}$, where $\mathbf{S}$ is the square MO overlap matrix defined in the main text for the case of two subsystems $A$ and $B$. We order elements of the MO overlap matrix $\mathbf{S}$ such that it is in a block-diagonal form,

$$\mathbf{S} = \begin{pmatrix} \mathbf{I}_A & \mathbf{S}_{AB} \\ \mathbf{S}_{BA} & \mathbf{I}_B \end{pmatrix}, \tag{2}$$

with $\mathbf{I}_A$ and $\mathbf{I}_B$ being identity matrices of sizes $[N_A \times N_A]$ and $[N_B \times N_B]$, respectively. The blocks $\mathbf{S}_{AB}$ and $\mathbf{S}_{BA}$ are of size $[N_A \times N_B]$ and $[N_B \times N_A]$, respectively, and contain overlaps between the MOs of subsystems $A$ and $B$, i.e., $(\mathbf{S}_{AB})_{ij} = \langle \psi_i^A | \psi_j^B \rangle$ and $(\mathbf{S}_{BA})_{ji} = \langle \psi_j^B | \psi_i^A \rangle$ with $i \in \{1, ..., N_A\}$, $j \in \{1, ..., N_B\}$. Using the fact that MOs belonging to the same subsystem are mutually orthonormal, i.e., $\langle \psi_i^I | \psi_j^I \rangle = \delta_{ij}$ for $I = A$ or $B$, the first four terms of the expansion from Eq. (1) become

$$\mathbf{A}^0 = \mathbf{I}, \tag{3}$$

$$\mathbf{A}^1 = \begin{pmatrix} \mathbf{0} & -\mathbf{S}_{AB} \\ -\mathbf{S}_{BA} & \mathbf{0} \end{pmatrix}, \tag{4}$$

$$\mathbf{A}^2 = \begin{pmatrix} \mathbf{S}_{AB}\mathbf{S}_{BA} & \mathbf{0} \\ \mathbf{0} & \mathbf{S}_{BA}\mathbf{S}_{AB} \end{pmatrix}, \tag{5}$$

and

$$\mathbf{A}^3 = \begin{pmatrix} \mathbf{0} & -\mathbf{S}_{AB}\mathbf{S}_{BA}\mathbf{S}_{AB} \\ -\mathbf{S}_{BA}\mathbf{S}_{AB}\mathbf{S}_{BA} & \mathbf{0} \end{pmatrix}. \tag{6}$$

Furthermore, we represent the matrix containing one-electron kinetic energy integrals $\mathbf{T}$ as

$$\mathbf{T} = \begin{pmatrix} \mathbf{T}_{AA} & \mathbf{T}_{AB} \\ \mathbf{T}_{BA} & \mathbf{T}_{BB} \end{pmatrix}, \tag{7}$$

with blocks $(\mathbf{T}_{IJ})_{ij} = \langle \psi_i^I | \hat{t} | \psi_j^J \rangle$, where $\hat{t}$ denotes the one-electron kinetic energy operator $-\nabla^2/2$ and $I, J = A$ or $B$. With these matrices being introduced, we can re-write the expression for the non-interactive kinetic energy $T_s$ of the total molecular system, as given in Eq. (11) in the main text, such that

$$T_s \approx \sum_{n=0}^{\infty} \sum_{i,j=1}^{N_A+N_B} (\mathbf{T})_{ij} (\mathbf{A}^n)_{ji} = \sum_{n=0}^{\infty} T_s^{(n)}. \tag{8}$$

Here, $T_s^{(n)}$ denotes the $n$th-order term of the expansion,

$$T_s^{(n)} := \sum_{i,j=1}^{N_A+N_B} (\mathbf{T})_{ij} \left( (\mathbf{I} - \mathbf{S})^n \right)_{ji}. \tag{9}$$

Substituting Eq. (3) in Eq. (8), we can obtain the expression for the zero-order term $T_s^{(0)}$. It reads

$$T_s^{(0)} = \sum_{i,j=1}^{N_A+N_B} (\mathbf{T})_{ij} \left( \mathbf{A}^0 \right)_{ji} = \sum_{i,j=1}^{N_A+N_B} (\mathbf{T})_{ij} \delta_{ij} = \sum_{I=A,B} \sum_{i=1}^{N_I} \langle \psi_i^I | \hat{t} | \psi_i^I \rangle = T_s[\{\psi_i^A\}] + T_s[\{\psi_i^B\}]. \tag{10}$$

Analogously, higher-order expansion terms can be expressed as

$$T_s^{(1)} = \sum_{i,j=1}^{N_A+N_B} (\mathbf{T})_{ij} \left(\mathbf{A}\right)_{ji} = -\sum_{i=1}^{N_A}\sum_{j=1}^{N_B}[(\mathbf{T}_{AB})_{ij}(\mathbf{S}_{BA})_{ji} + (\mathbf{T}_{BA})_{ji}(\mathbf{S}_{AB})_{ij}], \tag{11}$$

$$T_s^{(2)} = \sum_{i,j=1}^{N_A+N_B} (\mathbf{T})_{ij}(\mathbf{A}^2)_{ji} = \sum_{i,j=1}^{N_A}(\mathbf{T}_{AA})_{ij}(\mathbf{S}_{AB}\mathbf{S}_{BA})_{ji} + \sum_{i,j=1}^{N_B}(\mathbf{T}_{BB})_{ij}(\mathbf{S}_{BA}\mathbf{S}_{AB})_{ji}, \tag{12}$$

and

$$T_s^{(3)} = \sum_{i,j=1}^{N_A+N_B} (\mathbf{T})_{ij} \left(\mathbf{A}^3\right)_{ji} = -\sum_{i=1}^{N_A}\sum_{j=1}^{N_B}[(\mathbf{T}_{AB})_{ij}(\mathbf{S}_{BA}\mathbf{S}_{AB}\mathbf{S}_{BA})_{ji}+ (\mathbf{T}_{BA})_{ji}(\mathbf{S}_{AB}\mathbf{S}_{BA}\mathbf{S}_{AB})_{ij}]. \tag{13}$$

Introducing projection operators $\hat{\rho}_I$ of the form

$$\hat{\rho}_I = \sum_{i=1}^{N_I} |\psi_i^I\rangle \langle\psi_i^I| \,, \tag{14}$$

expressions in Eqs. (38)–(40) can further be simplified. Thus, for $T_s^{(1)}$ we have,

$$T_s^{(1)} = -\sum_{i=1}^{N_A}\sum_{j=1}^{N_B}[(\mathbf{T}_{AB})_{ij}(\mathbf{S}_{BA})_{ji} + (\mathbf{T}_{BA})_{ji}(\mathbf{S}_{AB})_{ij}] = -\sum_{i=1}^{N_A}\sum_{j=1}^{N_B}[\langle\psi_i^A|\hat{t}|\psi_j^B\rangle \langle\psi_j^B|\psi_i^A\rangle + \langle\psi_i^A|\psi_j^B\rangle \langle\psi_j^B|\hat{t}|\psi_i^A\rangle] = -\sum_{i=1}^{N_A}[\langle\psi_i^A|\hat{t}\hat{\rho}_B|\psi_i^A\rangle + \langle\psi_i^A|\hat{\rho}_B\hat{t}|\psi_i^A\rangle] = -\sum_{i=1}^{N_A} \langle\psi_i^A|\hat{t}\hat{\rho}_B + \hat{\rho}_B\hat{t}|\psi_i^A\rangle \,. \tag{15}$$

Similarly, the expression for $T_s^{(2)}$ is derived, resulting in

$$
\begin{aligned}
T_s^{(2)} &= \sum_{i,j=1}^{N_A} (\mathbf{T}_{AA})_{ij} (\mathbf{S}_{AB}\mathbf{S}_{BA})_{ji} + \sum_{i,j=1}^{N_B} (\mathbf{T}_{BB})_{ij} (\mathbf{S}_{BA}\mathbf{S}_{AB})_{ji} = \\
&\sum_{i,j=1}^{N_A} \sum_{k=1}^{N_B} \langle \psi_i^A | \hat{t} | \psi_j^A \rangle \langle \psi_j^A | \psi_k^B \rangle \langle \psi_k^B | \psi_i^A \rangle + \sum_{i,j=1}^{N_B} \sum_{k=1}^{N_A} \langle \psi_k^A | \psi_i^B \rangle \langle \psi_i^B | \hat{t} | \psi_j^B \rangle \langle \psi_j^B | \psi_k^A \rangle = \\
&\quad \frac{1}{2} \sum_{i=1}^{N_A} \langle \psi_i^A | \hat{t} \hat{\rho}_A \hat{\rho}_B | \psi_i^A \rangle + \frac{1}{2} \sum_{j=1}^{N_A} \langle \psi_j^A | \hat{\rho}_B \hat{\rho}_A \hat{t} | \psi_j^A \rangle + \sum_{k=1}^{N_A} \langle \psi_k^A | \hat{\rho}_B \hat{t} \hat{\rho}_B | \psi_k^A \rangle = \\
&\qquad \frac{1}{2} \sum_{i=1}^{N_A} \langle \psi_i^A | \hat{t} \hat{\rho}_A \hat{\rho}_B + \hat{\rho}_B \hat{\rho}_A \hat{t} + 2 \hat{\rho}_B \hat{t} \hat{\rho}_B | \psi_i^A \rangle \, . \qquad (16)
\end{aligned}
$$

Note that the term $\sum_{i,j=1}^{N_A} (\mathbf{T}_{AA})_{ij} (\mathbf{S}_{AB}\mathbf{S}_{BA})_{ji}$ was written here as an averaged sum of two equivalent expressions to ensure Hermiticity of the resulting operator $\hat{t}\hat{\rho}_A\hat{\rho}_B + \hat{\rho}_B\hat{\rho}_A\hat{t} + 2\hat{\rho}_B\hat{t}\hat{\rho}_B$.

Finally, for $T_s^{(3)}$ one obtains,

$$
\begin{aligned}
T_s^{(3)} &= - \sum_{i=1}^{N_A} \sum_{j=1}^{N_B} [(\mathbf{T}_{AB})_{ij} (\mathbf{S}_{BA}\mathbf{S}_{AB}\mathbf{S}_{BA})_{ji} + (\mathbf{T}_{BA})_{ji} (\mathbf{S}_{AB}\mathbf{S}_{BA}\mathbf{S}_{AB})_{ij}] = \\
&\quad - \frac{1}{2} \sum_{i=1}^{N_A} \langle \psi_i^A | \hat{t} \hat{\rho}_B \hat{\rho}_A \hat{\rho}_B + \hat{\rho}_B \hat{t} \hat{\rho}_A \hat{\rho}_B + \hat{\rho}_B \hat{\rho}_A \hat{t} \hat{\rho}_B + \hat{\rho}_B \hat{\rho}_A \hat{\rho}_B \hat{t} | \psi_i^A \rangle \, . \qquad (17)
\end{aligned}
$$

# S2 Functional Derivatives

Derivations presented in this section follow closely definitions and notations from Ref. [3]. A mathematically more rigorous description of the theory of functional derivatives could be found in Ref. [4].

## S2.1 Formal Definition and Notations

We define a functional $F[f]$ as a rule associating a real or complex number with a function $f(x)$ and subsequently define a functional variation $\delta F[f]$ as

$$\delta F[f] \coloneqq F[f+\delta f] - F[f] = F[f+\epsilon\eta] - F[f]. \tag{18}$$

Here, the function $f(x)$ is varied by $\delta f = \epsilon\eta$, where $\epsilon$ is an infinitesimal number and $\eta(x)$ is an arbitrary function. Expanding $F[f+\epsilon\eta]$ in a Taylor series in powers of $\epsilon$, we obtain

$$F[f+\epsilon\eta] = F[f] + \left.\frac{\mathrm{d}F[f+\epsilon\eta]}{\mathrm{d}\epsilon}\right|_{\epsilon=0} \epsilon + O(\epsilon^2). \tag{19}$$

Considering only the second term of this expansion, one could define the functional derivative $\delta F[f]/\delta f(x)$ such that

$$\int \frac{\delta F[f]}{\delta f(x)} \delta\eta(x)\mathrm{d}x \coloneqq \left.\frac{\mathrm{d}F[f+\epsilon\eta]}{\mathrm{d}\epsilon}\right|_{\epsilon=0}. \tag{20}$$

Finally, comparing Eqs. (18–20), a relation between the functional variation $\delta F[f]$ and the functional derivative $\delta F[f]/\delta f(x)$ could be established,

$$\delta F[f] \approx \epsilon \int \frac{\delta F[f]}{\delta f(x)} \delta\eta(x)\mathrm{d}x. \tag{21}$$

A similar expression could be obtained for functionals of many functions $F[f_1, f_2, \ldots, f_m]$ (see Ref. [4]), i.e.,

$$\delta F[f_1, f_2, \ldots, f_m] \approx \sum_{i=1}^{m} \int \frac{\delta F[f_1, f_2, \ldots, f_m]}{\delta f_i(x)} \delta f_i(x)\mathrm{d}x. \tag{22}$$

## S2.2 Functional Derivatives of Kinetic Energy Contributions

In the following, we consider kinetic energy contributions as functionals of MOs, e.g., $T_s = T_s[\{\psi_i^A\},\{\psi_i^B\}]$, and apply Eqs. (21) and (22) for evaluations of corresponding functional derivatives.

In the case of $T_s^{(1)}$, given in Eq. (38), the corresponding variation $\delta T_s^{(1)}$ is given as

$$\begin{aligned}\delta T_s^{(1)} = -\sum_{i=1}^{N_A}\sum_{j=1}^{N_B}[&\langle\delta\psi_i^A|\hat{t}|\psi_j^B\rangle\langle\psi_j^B|\psi_i^A\rangle + \langle\psi_i^A|\hat{t}|\delta\psi_j^B\rangle\langle\psi_j^B|\psi_i^A\rangle \\ &+ \langle\psi_i^A|\hat{t}|\psi_j^B\rangle\langle\delta\psi_j^B|\psi_i^A\rangle + \langle\psi_i^A|\hat{t}|\psi_j^B\rangle\langle\psi_j^B|\delta\psi_i^A\rangle \\ &+ \langle\delta\psi_j^B|\hat{t}|\psi_i^A\rangle\langle\psi_i^A|\psi_j^B\rangle + \langle\psi_j^B|\hat{t}|\delta\psi_i^A\rangle\langle\psi_i^A|\psi_j^B\rangle \\ &+ \langle\psi_j^B|\hat{t}|\psi_i^A\rangle\langle\delta\psi_i^A|\psi_j^B\rangle + \langle\psi_j^B|\hat{t}|\psi_i^A\rangle\langle\psi_i^A|\delta\psi_j^B\rangle].\end{aligned} \tag{23}$$

Comparing Eqs. (22) and (23), one can see that only the first and seventh summands of Eq. (23) lead to non-zero contributions to the functional derivative of $T_s^{(1)}$ with respect to a specific $\psi_l^{A*}$, $l \in \{1,...,N_A\}$. Using the projection operators $\hat{\rho}_I$ introduced in Eq. (14), the functional derivative of $T_s^{(1)}$ with respect to $\psi_l^{A*}$ can be re-written as

$$\frac{\delta T_s^{(1)}}{\delta\psi_l^{A*}} = -(\hat{\rho}_B\hat{t} + \hat{t}\hat{\rho}_B)\psi_l^A. \tag{24}$$

For $T_s^{(2)}$ and $T_s^{(3)}$, the functional variations can be taken in full analogy to the example above. This leads to functional derivatives of the form,

$$\frac{\delta T_s^{(2)}}{\delta\psi_l^{A*}} = \left(\hat{\rho}_B\hat{\rho}_A\hat{t} + \hat{t}\hat{\rho}_A\hat{\rho}_B + \hat{\rho}_B\hat{t}\hat{\rho}_B\right)\psi_l^A \tag{25}$$

and

$$\frac{\delta T_s^{(3)}}{\delta\psi_l^{A*}} = -\left(\hat{t}\hat{\rho}_B\hat{\rho}_A\hat{\rho}_B + \hat{\rho}_B\hat{t}\hat{\rho}_A\hat{\rho}_B + \hat{\rho}_B\hat{\rho}_A\hat{t}\hat{\rho}_B + \hat{\rho}_B\hat{\rho}_A\hat{\rho}_B\hat{t}\right)\psi_l^A. \tag{26}$$

# S3 Equations in Atomic-Orbital Representation

## S3.1 Non-Additive Kinetic Contributions

In the case of restricted computations, operators from Eqs. (24)–(26) could be written in atomic-orbital (AO) representation such that

$$\mathbf{T}^{(1),\mathrm{AO}} = -a\left(\mathbf{S}^{\mathrm{AO}}_{AB}\mathbf{P}_{BB}\mathbf{T}^{\mathrm{AO}}_{BA} + \mathbf{T}^{\mathrm{AO}}_{AB}\mathbf{P}_{BB}\mathbf{S}^{\mathrm{AO}}_{BA}\right), \tag{27}$$

$$\begin{aligned}\mathbf{T}^{(2),\mathrm{AO}} = a^2(&\mathbf{S}^{\mathrm{AO}}_{AB}\mathbf{P}_{BB}\mathbf{S}^{\mathrm{AO}}_{BA}\mathbf{P}_{AA}\mathbf{T}^{\mathrm{AO}}_{AA} + \mathbf{T}^{\mathrm{AO}}_{AA}\mathbf{P}_{AA}\mathbf{S}^{\mathrm{AO}}_{AB}\mathbf{P}_{BB}\mathbf{S}^{\mathrm{AO}}_{BA} +\\ &\mathbf{S}^{\mathrm{AO}}_{AB}\mathbf{P}_{BB}\mathbf{T}^{\mathrm{AO}}_{BB}\mathbf{P}_{BB}\mathbf{S}^{\mathrm{AO}}_{BA}),\end{aligned} \tag{28}$$

$$\begin{aligned}\mathbf{T}^{(3),\mathrm{AO}} = -a^3(&\mathbf{T}^{\mathrm{AO}}_{AB}\mathbf{P}_{BB}\mathbf{S}^{\mathrm{AO}}_{BA}\mathbf{P}_{AA}\mathbf{S}^{\mathrm{AO}}_{AB}\mathbf{P}_{BB}\mathbf{S}^{\mathrm{AO}}_{BA} + \mathbf{S}^{\mathrm{AO}}_{AB}\mathbf{P}_{BB}\mathbf{S}^{\mathrm{AO}}_{BA}\mathbf{P}_{AA}\mathbf{S}^{\mathrm{AO}}_{AB}\mathbf{P}_{BB}\mathbf{T}^{\mathrm{AO}}_{BA} +\\ &\mathbf{S}^{\mathrm{AO}}_{AB}\mathbf{P}_{BB}\mathbf{T}^{\mathrm{AO}}_{BA}\mathbf{P}_{AA}\mathbf{S}^{\mathrm{AO}}_{AB}\mathbf{P}_{BB}\mathbf{S}^{\mathrm{AO}}_{BA} + \mathbf{S}^{\mathrm{AO}}_{AB}\mathbf{P}_{BB}\mathbf{S}^{\mathrm{AO}}_{BA}\mathbf{P}_{AA}\mathbf{T}^{\mathrm{AO}}_{AB}\mathbf{P}_{BB}\mathbf{S}^{\mathrm{AO}}_{BA}).\end{aligned} \tag{29}$$

Here, $a$ is a multiplicative prefactor, which is equal to 1/2 and originates from the fact that the density matrices $\mathbf{P}_{AA}$ and $\mathbf{P}_{BB}$ contain a factor of two,

$$(\mathbf{P}_{II})_{\mu\nu} = 2\sum_{i=1}^{N_I/2} c^I_{\mu i}c^I_{\nu i}. \tag{30}$$

In Eq. (30), $c^I_{\mu i}$ are the MO coefficients of subsystem $I$ and $\mu, \nu \in \{1, ..., n_I\}$ with $n_I$ being the number of AOs describing subsystem $I$. $\mathbf{S}^{\mathrm{AO}}_{AB}$ is the AO overlap matrix with elements

$$\left(\mathbf{S}^{\mathrm{AO}}_{AB}\right)_{\mu\nu} = \langle\chi^A_\mu|\chi^B_\nu\rangle \tag{31}$$

where $\chi_\mu^A$ and $\chi_\nu^B$ are AOs belonging to subsystems $A$ and $B$, respectively. Since real AOs are used, $(\mathbf{S}_{AB}^{\text{AO}})^T = \mathbf{S}_{BA}^{\text{AO}}$. Furthermore, the matrix blocks $\mathbf{T}_{IJ}^{\text{AO}}$ contain the one-electron kinetic energy integrals, namely

$$\left(\mathbf{T}_{IJ}^{\text{AO}}\right)_{\mu\nu} = \langle \chi_\mu^I | \hat{t} | \chi_\nu^J \rangle \,. \tag{32}$$

Note that the expressions in Eqs. (27)–(29) are used to construct the Fock matrix of the active subsystem $A$ and self-consistently account for the non-additivity of the kinetic energy. In order to compute the corresponding energy contributions, the following expressions could be used:

$$T_s^{(1)} = \sum_{\mu,\nu} \left(\mathbf{P}_{AA}\right)_{\mu\nu} \left(\mathbf{T}^{(1),\text{AO}}\right)_{\mu\nu} , \tag{33}$$

$$T_s^{(2)} = \sum_{\mu,\nu} \left(\mathbf{P}_{AA}\right)_{\mu\nu} (\mathbf{T}^{(2),\text{AO}} - \frac{1}{2} a^2 \mathbf{S}_{AB}^{\text{AO}} \mathbf{P}_{BB} \mathbf{S}_{BA}^{\text{AO}} \mathbf{P}_{AA} \mathbf{T}_{AA}^{\text{AO}} - \frac{1}{2} a^2 \mathbf{T}_{AA}^{\text{AO}} \mathbf{P}_{AA} \mathbf{S}_{AB}^{\text{AO}} \mathbf{P}_{BB} \mathbf{S}_{BA}^{\text{AO}})_{\mu\nu}, \tag{34}$$

$$T_s^{(3)} = \frac{1}{2} \sum_{\mu,\nu} \left(\mathbf{P}_{AA}\right)_{\mu\nu} \left(\mathbf{T}^{(3),\text{AO}}\right)_{\mu\nu} . \tag{35}$$

Here, additional terms on the right-hand side of Eq. (34) appear due to the difference between operator expressions in Eqs. (16) and (25). For similar reasons, a prefactor of 1/2 is inserted in Eq. (35).

The direct evaluation of expansion terms as given in Eqs. (27)–(29) involves many matrix–matrix multiplications and is, therefore, very costly. However, analyzing these expressions, one can notice that several matrix products appear multiple times and can be evaluated, stored, and re-used. Furthermore, each expression involves terms, which are transposed

of each other. Taking this into account, we introduced the following matrix products

$$\mathbf{K}_{AB} = \mathbf{S}^{\text{AO}}_{AB}\mathbf{P}_{BB} \qquad \mathbf{L}_{AA} = \mathbf{K}_{AB}\mathbf{T}^{\text{AO}}_{BA} \tag{36}$$

$$\mathbf{M}_{AB} = \mathbf{P}_{AA}\mathbf{S}^{\text{AO}}_{AB} \qquad \mathbf{N}_{AA} = \mathbf{K}_{AB}\mathbf{M}_{BA} \tag{37}$$

and denoted the corresponding transposed matrices as $\mathbf{K}_{BA}$, $(\mathbf{L}_{AA})^{\text{T}}$, $\mathbf{M}_{BA}$, and $(\mathbf{N}_{AA})^{\text{T}}$, respectively. Then, expressions for the expansion terms $\mathbf{T}^{(1),\text{AO}}$, $\mathbf{T}^{(2),\text{AO}}$, and $\mathbf{T}^{(3),\text{AO}}$ read

$$\mathbf{T}^{(1),\text{AO}} = -a\left[\mathbf{L}_{AA} + (\mathbf{L}_{AA})^{\text{T}}\right], \tag{38}$$

$$\mathbf{T}^{(2),\text{AO}} = a^2\left[\mathbf{N}_{AA}\mathbf{T}_{AA} + (\mathbf{N}_{AA}\mathbf{T}_{AA})^{\text{T}} + \mathbf{K}_{AB}\mathbf{T}_{BB}\mathbf{K}_{BA}\right], \tag{39}$$

and

$$\mathbf{T}^{(3),\text{AO}} = -a^3\left[\mathbf{N}_{AA}\mathbf{L}_{AA} + (\mathbf{N}_{AA}\mathbf{L}_{AA})^{\text{T}} + \mathbf{N}_{AA}(\mathbf{L}_{AA})^{\text{T}} + (\mathbf{N}_{AA}(\mathbf{L}_{AA})^{\text{T}})^{\text{T}}\right], \tag{40}$$

respectively. Therefore, evaluations of $\mathbf{T}^{(1),\text{AO}}$ require computations of only two matrix products from Eq. (36). In the case of the series being truncated at the second order, $\mathbf{T}^{(1),\text{AO}}$ and $\mathbf{T}^{(2),\text{AO}}$ are computed by performing seven matrix–matrix multiplications in total. For the third-order truncated series, eleven multiplications are required. Their computational cost is summarized in Tab. S1. Finally, the energy expression from Eq. (34)

| Order of truncation, $M$ | Dominating terms |
|---|---|
| 1 | $n_A^2 n_B$, $n_A n_B^2$ |
| 2 | $n_A^3$, $n_A^2 n_B$, $n_A n_B^2$ |
| 3 | $n_A^3$, $n_A^2 n_B$, $n_A n_B^2$ |

Table S1: Dominating contributions to the computational cost of evaluating non-additive kinetic energy terms. $n_A$ and $n_B$ are the number of AOs of subsystem $A$ and $B$, respectively.

becomes

$$T_s^{(2)} = \sum_{\mu,\nu} (\mathbf{P}_{AA})_{\mu\nu} \left( \mathbf{T}^{(2),\mathrm{AO}} - \frac{1}{2} a^2 \mathbf{N}_{AA} \mathbf{T}_{AA}^{\mathrm{AO}} - \frac{1}{2} a^2 (\mathbf{N}_{AA} \mathbf{T}_{AA}^{\mathrm{AO}})^{\mathrm{T}} \right)_{\mu\nu} . \tag{41}$$

## S3.2 Non-Additive Exchange–Correlation Contributions

As discussed in the main text, the only component required for approximating the non-additive XC energy contribution is the electron density $\rho_\Phi(\vec{r})$, which is described by the density matrix $\mathbf{P}_\Phi$ in AO representation. In order to derive the expression for $\mathbf{P}_\Phi$, we start from Eq. (24) from the main text and carry out integration of the $\langle \phi_i | \delta(\vec{r}_i - \vec{r}) | \phi_j \rangle$ terms, which results in

$$\rho_\Phi(\vec{r}) = \sum_{i,j=1}^{N_A+N_B} \phi_i \phi_j (\mathbf{S}^{-1})_{ji}. \tag{42}$$

This expression could be re-written in a matrix form as

$$\rho_\Phi = \boldsymbol{\phi}^{\mathrm{T}} \mathbf{S}^{-1} \boldsymbol{\phi}, \tag{43}$$

where $\boldsymbol{\phi}$ is a column vector containing MOs of the entire molecular system

$$\boldsymbol{\phi} = \begin{pmatrix} \boldsymbol{\psi}^A \\ \boldsymbol{\psi}^B \end{pmatrix} = \begin{pmatrix} \psi_1^A \\ \vdots \\ \psi_{N_A}^A \\ \psi_1^B \\ \vdots \\ \psi_{N_B}^B \end{pmatrix} . \tag{44}$$

Expanding the column vector of MOs into a linear combination of AOs, we arrive at the equation,

$$\rho_\Phi = (\mathbf{C}^{\mathrm{T}} \boldsymbol{\chi})^{\mathrm{T}} \mathbf{S}^{-1} \mathbf{C}^{\mathrm{T}} \boldsymbol{\chi}, \tag{45}$$

where $\mathbf{C}$ denote block-diagonal matrices of MO coefficients,

$$\mathbf{C} = \begin{pmatrix} \mathbf{C}_A & \mathbf{0} \\ \mathbf{0} & \mathbf{C}_B \end{pmatrix} \tag{46}$$

and $\boldsymbol{\chi}$ is a column vector of AOs. From Eq. (45), it follows that the density matrix $\mathbf{P}_\Phi$ is given as

$$\mathbf{P}_\Phi = \mathbf{C}\mathbf{S}^{-1}\mathbf{C}^{\mathrm{T}}. \tag{47}$$

Denoting blocks of the inverse MO overlap matrix such that

$$\mathbf{S}^{-1} = \begin{pmatrix} \tilde{\mathbf{S}}_{AA} & \tilde{\mathbf{S}}_{AB} \\ \tilde{\mathbf{S}}_{BA} & \tilde{\mathbf{S}}_{BB} \end{pmatrix} \tag{48}$$

and substituting Eq. (48) into Eq. (47), we obtain,

$$\mathbf{P}_\Phi = \begin{pmatrix} \mathbf{C}_A\tilde{\mathbf{S}}_{AA}\mathbf{C}_A^{\mathrm{T}} & \mathbf{C}_A\tilde{\mathbf{S}}_{AB}\mathbf{C}_B^{\mathrm{T}} \\ \mathbf{C}_B\tilde{\mathbf{S}}_{BA}\mathbf{C}_A^{\mathrm{T}} & \mathbf{C}_B\tilde{\mathbf{S}}_{BB}\mathbf{C}_B^{\mathrm{T}} \end{pmatrix}. \tag{49}$$

Expanding the inverse MO overlap matrix $\mathbf{S}^{-1}$ into the Neumann series, we can finally express the density matrix $\mathbf{P}_\Phi$ as the sum of correction terms,

$$\mathbf{P}_\Phi = \mathbf{P}^{(0)} + \mathbf{P}^{(1)} + \mathbf{P}^{(2)} + \dots \tag{50}$$

where

$$\mathbf{P}^{(0)} = \begin{pmatrix} \mathbf{P}_{AA} & \mathbf{0} \\ \mathbf{0} & \mathbf{P}_{BB} \end{pmatrix}, \tag{51}$$

$$\mathbf{P}^{(1)} = \begin{pmatrix} \mathbf{0} & -\mathbf{P}_{AA}\mathbf{S}^{\mathrm{AO}}_{AB}\mathbf{P}_{BB} \\ -\mathbf{P}_{BB}\mathbf{S}^{\mathrm{AO}}_{BA}\mathbf{P}_{AA} & \mathbf{0} \end{pmatrix}, \tag{52}$$

and

$$\mathbf{P}^{(2)} = \begin{pmatrix} \mathbf{P}_{AA}\mathbf{S}^{\mathrm{AO}}_{AB}\mathbf{P}_{BB}\mathbf{S}^{\mathrm{AO}}_{BA}\mathbf{P}_{AA} & \mathbf{0} \\ \mathbf{0} & \mathbf{P}_{BB}\mathbf{S}^{\mathrm{AO}}_{BA}\mathbf{P}_{AA}\mathbf{S}^{\mathrm{AO}}_{AB}\mathbf{P}_{BB} \end{pmatrix}. \tag{53}$$

The computational cost associated with computing $\mathbf{P}^{(1)}$ and $\mathbf{P}^{(2)}$ is summarized in Tab. S2.

| Order of truncation, $M$ | Dominating terms |
|---|---|
| 1 | $n_A^2 n_B$, $n_A n_B^2$ |
| 2 | $n_A^3$, $n_B^3$ |

Table S2: Dominating contributions to the computational cost of evaluating density matrix correction terms. $n_A$ and $n_B$ are the number of AOs of subsystem $A$ and $B$, respectively.

## S3.3 Alternative Expressions for Kinetic Energy Terms

It is interesting to note that the definition of the density matrix $\mathbf{P}_\Phi$ from Sec. S3.2 could be used to provide alternative expressions for kinetic energies given in Sec. S3.1. To that end, we note that the kinetic energy of the total molecular system is equal to

$$T_s = \sum_{\mu\nu} \mathbf{T}^{\mathrm{AO}}_{\mu\nu} (\mathbf{P}_\Phi)_{\mu\nu}, \tag{54}$$

where $\mathbf{T}^{\mathrm{AO}}$ is the matrix of kinetic energy integrals of the total system,

$$\mathbf{T}^{\mathrm{AO}} = \begin{pmatrix} \mathbf{T}^{\mathrm{AO}}_{AA} & \mathbf{T}^{\mathrm{AO}}_{AB} \\ \mathbf{T}^{\mathrm{AO}}_{BA} & \mathbf{T}^{\mathrm{AO}}_{BB} \end{pmatrix} \tag{55}$$

containing matrix elements $(\mathbf{T}^{\mathrm{AO}}_{IJ})_{\mu\nu} = \langle \chi^I_\mu | \hat{t} | \chi^J_\nu \rangle$. Therefore, substituting the expanded density matrix expression from Eq. (50) into Eq. (54), we obtain the first three correction

terms,

$$T_s^{(0)} = \sum_{\mu\nu} \mathbf{T}^{\text{AO}}_{\mu\nu} \mathbf{P}^{(0)}_{\mu\nu} = \sum_{\mu\nu} (\mathbf{T}^{\text{AO}}_{AA})_{\mu\nu} (\mathbf{P}_{AA})_{\mu\nu} + \sum_{\mu\nu} (\mathbf{T}^{\text{AO}}_{BB})_{\mu\nu} (\mathbf{P}_{BB})_{\mu\nu}, \tag{56}$$

$$T_s^{(1)} = \sum_{\mu\nu} \mathbf{T}^{\text{AO}}_{\mu\nu} \mathbf{P}^{(1)}_{\mu\nu} = -\sum_{\mu\nu} (\mathbf{T}^{\text{AO}}_{AB})_{\mu\nu} (\mathbf{P}_{AA} \mathbf{S}^{\text{AO}}_{AB} \mathbf{P}_{BB})_{\mu\nu} - \sum_{\mu\nu} (\mathbf{T}^{\text{AO}}_{BA})_{\mu\nu} (\mathbf{P}_{BB} \mathbf{S}^{\text{AO}}_{BA} \mathbf{P}_{AA})_{\mu\nu}, \tag{57}$$

$$T_s^{(2)} = \sum_{\mu\nu} \mathbf{T}^{\text{AO}}_{\mu\nu} \mathbf{P}^{(2)}_{\mu\nu} = \sum_{\mu\nu} (\mathbf{T}^{\text{AO}}_{AA})_{\mu\nu} (\mathbf{P}_{AA} \mathbf{S}^{\text{AO}}_{AB} \mathbf{P}_{BB} \mathbf{S}^{\text{AO}}_{BA} \mathbf{P}_{AA})_{\mu\nu} + \sum_{\mu\nu} (\mathbf{T}^{\text{AO}}_{BB})_{\mu\nu} (\mathbf{P}_{BB} \mathbf{S}^{\text{AO}}_{BA} \mathbf{P}_{AA} \mathbf{S}^{\text{AO}}_{AB} \mathbf{P}_{BB})_{\mu\nu}. \tag{58}$$

Unfortunately, this formulation does not provide a simpler route for the computation of functional derivatives.

# S4 Matrix Norms

Norms are functions which assign non-negative real numbers to objects in vector spaces and applying a norm can be viewed as measuring the size of an element. Formally, a norm on a vector space $V$ over a field $\mathbb{K}$ of real $\mathbb{R}$ or complex $\mathbb{C}$ numbers is a function $\|\cdot\| : V \to \mathbb{R}$ with the following properties [5]:

1. positive definiteness: $\|x\| \geq 0$ and $\|x\| = 0 \iff x = 0$;
2. triangle-inequality: $\|x + y\| \leq \|x\| + \|y\|$;
3. absolute homogeneity: $\|\lambda x\| = |\lambda| \cdot \|x\|$;

for all $x, y \in V$, $\lambda \in \mathbb{K}$, and $|\cdot|$ denoting the absolute value.

The positive definiteness ensures that objects cannot have negative size. Furthermore, the zero element of the vector space should be the only element with zero size. The triangle-inequality states that "the direct way is always the shortest". Last, absolute homogeneity guarantees that scaling a vector also scales its size accordingly.

A matrix norm is a norm on $\mathbb{K}^{n\times m}$ with $n$ and $m$ being natural numbers. The following matrix norms for a (not necessarily square) real or complex matrix $\mathbf{M}$ with elements $(\mathbf{M})_{ij}$ were tested in this work:

1. The *1-norm* or *column sum norm* is given by the maximal sum over the absolute values of elements within a column of $\mathbf{M}$, namely

$$\|\mathbf{M}\|_1 = \max_{1\leq j\leq m} \sum_{i=1}^{n} |(\mathbf{M})_{ij}|. \tag{59}$$

2. The $\infty$-*norm* or *row sum norm* of $\mathbf{M}$ is given as the maximal sum over the absolute values of elements within a row of $\mathbf{M}$,

$$\|\mathbf{M}\|_\infty = \max_{1\leq i\leq n} \sum_{j=1}^{m} |(\mathbf{M})_{ij}|. \tag{60}$$

3. The *2-norm* or *spectral norm* of $\mathbf{M}$ can be expressed as the largest singular value $\sigma_{\max}$ of $\mathbf{M}$, i.e.,

$$\|\mathbf{M}\|_2 = \sigma_{\max}(\mathbf{M}). \tag{61}$$

4. The *Frobenius norm* of $\mathbf{M}$ is defined as the square root of the sum over all absolute square values of elements of $\mathbf{M}$, i.e.,

$$\|\mathbf{M}\|_F = \sqrt{\sum_{i=1}^{n}\sum_{j=1}^{m} |(\mathbf{M})_{ij}|^2}. \tag{62}$$

It should be noted that the 1-norm and $\infty$-norm are equivalent when applied to a sym-

metric matrix such as matrices $\mathbf{S}^{-1} - \sum_{n=0}^{M}(\mathbf{I} - \mathbf{S})^n$ studied in the main text. Therefore, results for the 1-norm and $\infty$-norm are not presented separately.

## S4.1 Comparing Different Norms

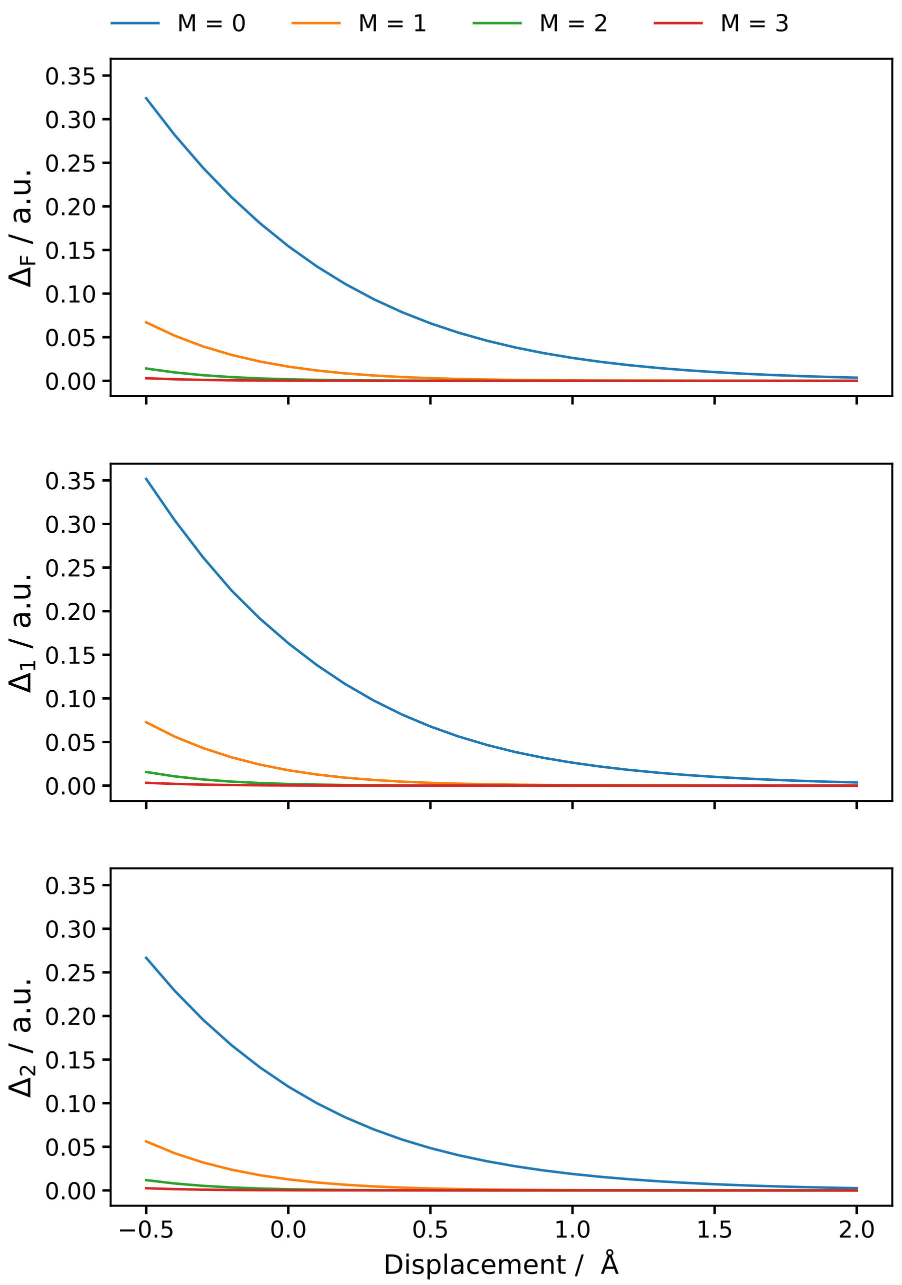


Figure S1: The error $\Delta$ computed at truncation levels $M = 0, 1, 2$, and 3 of the Neumann series. The results are shown for the molecular cluster $H_2O \cdots H_2O$ using the Frobenius norm $\Delta_F$ (top), 1-norm $\Delta_1$ (middle), and 2-norm $\Delta_2$ (bottom) at different intermolecular displacements relative to the equilibrium structure. Computations of overlap matrices were performed with sDFT using the kinetic energy functional PW91k.

# S5 Number of Electrons

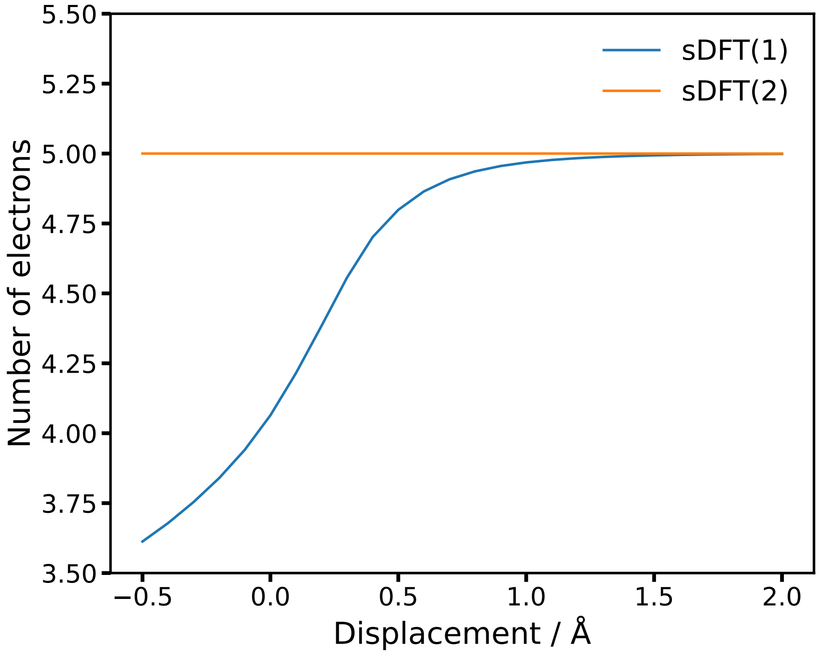


Figure S2: Integral of density $\rho_\Phi(\vec{r})$ as a function of intermolecular displacements between $Be^+$ and $H_2$ computed with sDFT($M$). The curves correspond to different truncation orders $M$ of the Neumann expansion.

# S6 Basis Set and Functional Dependence

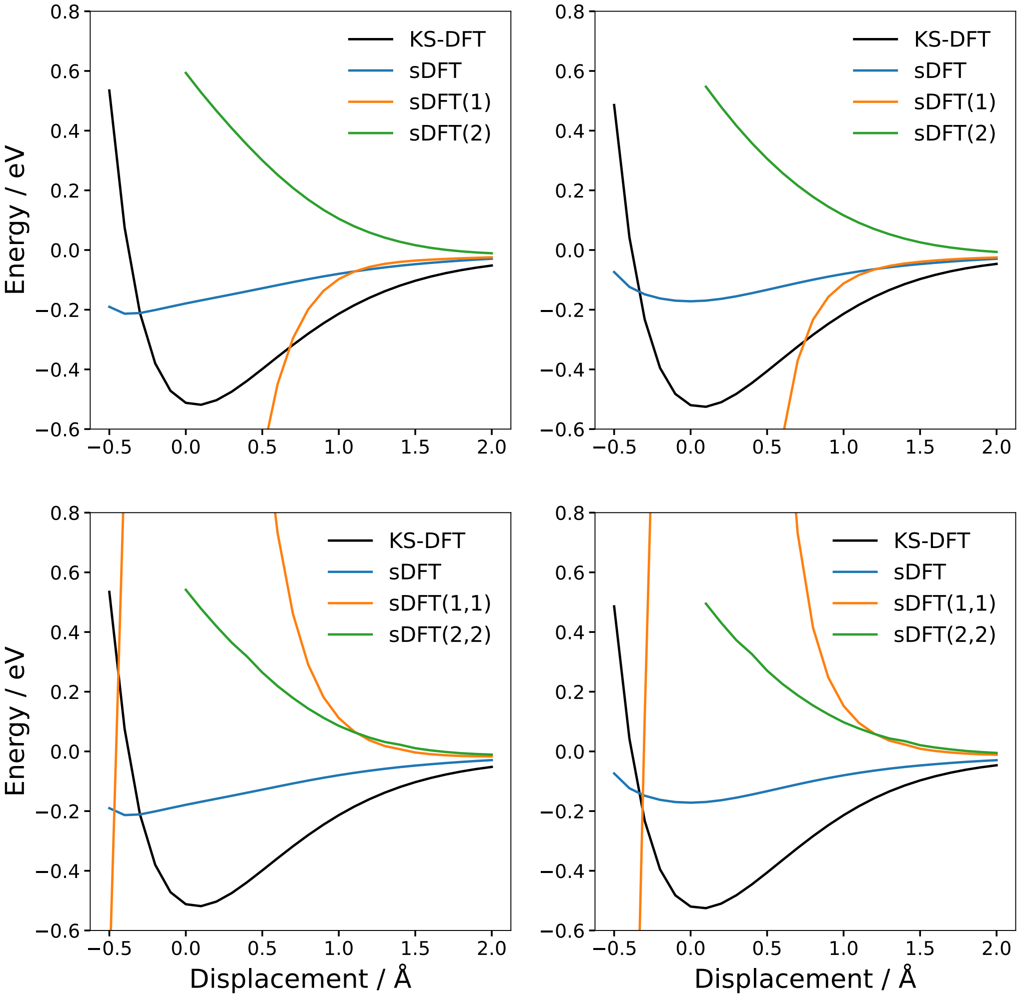


Figure S3: Interaction energies as functions of the intermolecular displacement computed for the $Be^{+} \cdots H_2$ complex with KS-DFT and sDFT-based approaches and using the PW91 XC functional. The basis sets def2-SVP and def2-TZVP were applied for the graphs on the left and on the right, respectively. The PW91k kinetic energy functional was used in sDFT computations.

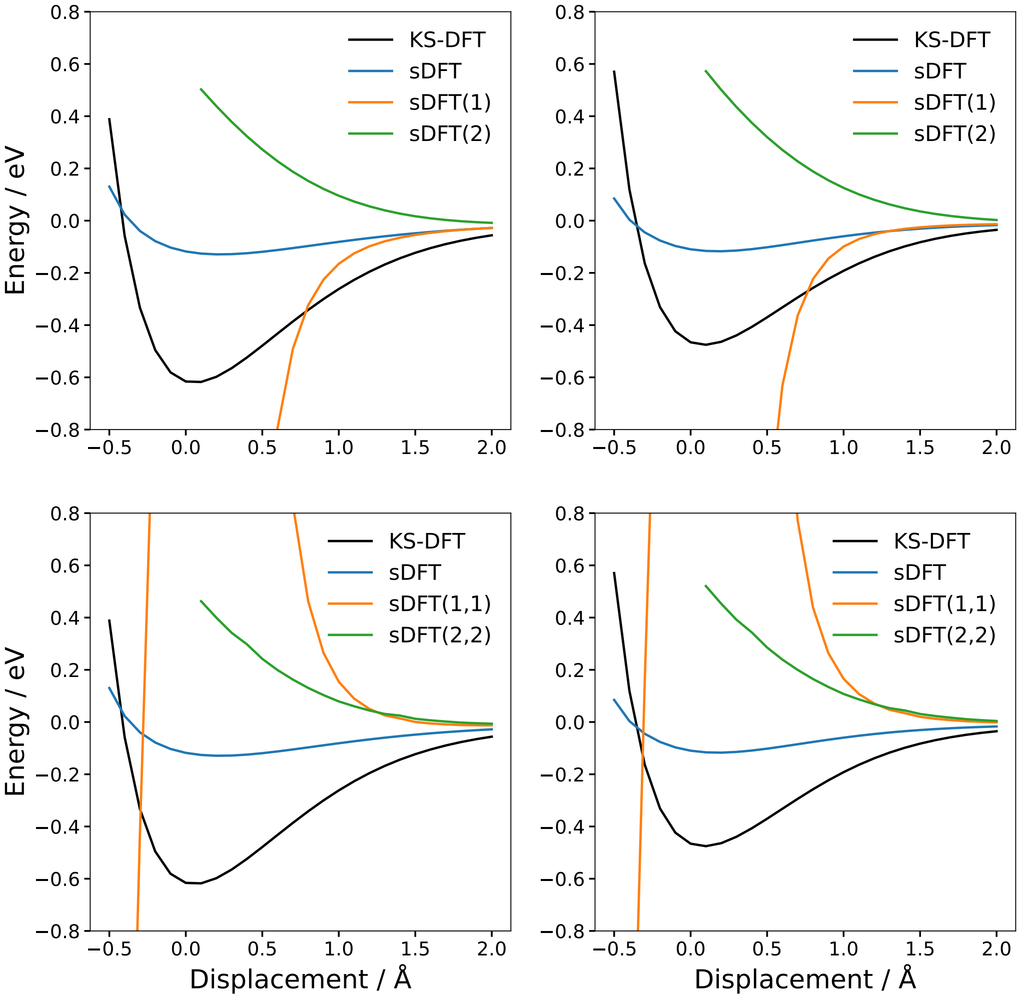


Figure S4: Interaction energies as functions of the intermolecular displacement computed for the $Be^{+} \cdots H_2$ complex with KS-DFT and sDFT-based approaches using the def2-TZVP basis set. The functionals LDA and BP86 were applied for the graphs on the left and on the right, respectively. In sDFT computations, the TF and LLP91K functionals were used in conjunction with LDA and BP86, respectively.

# S7 Integrated Density Errors

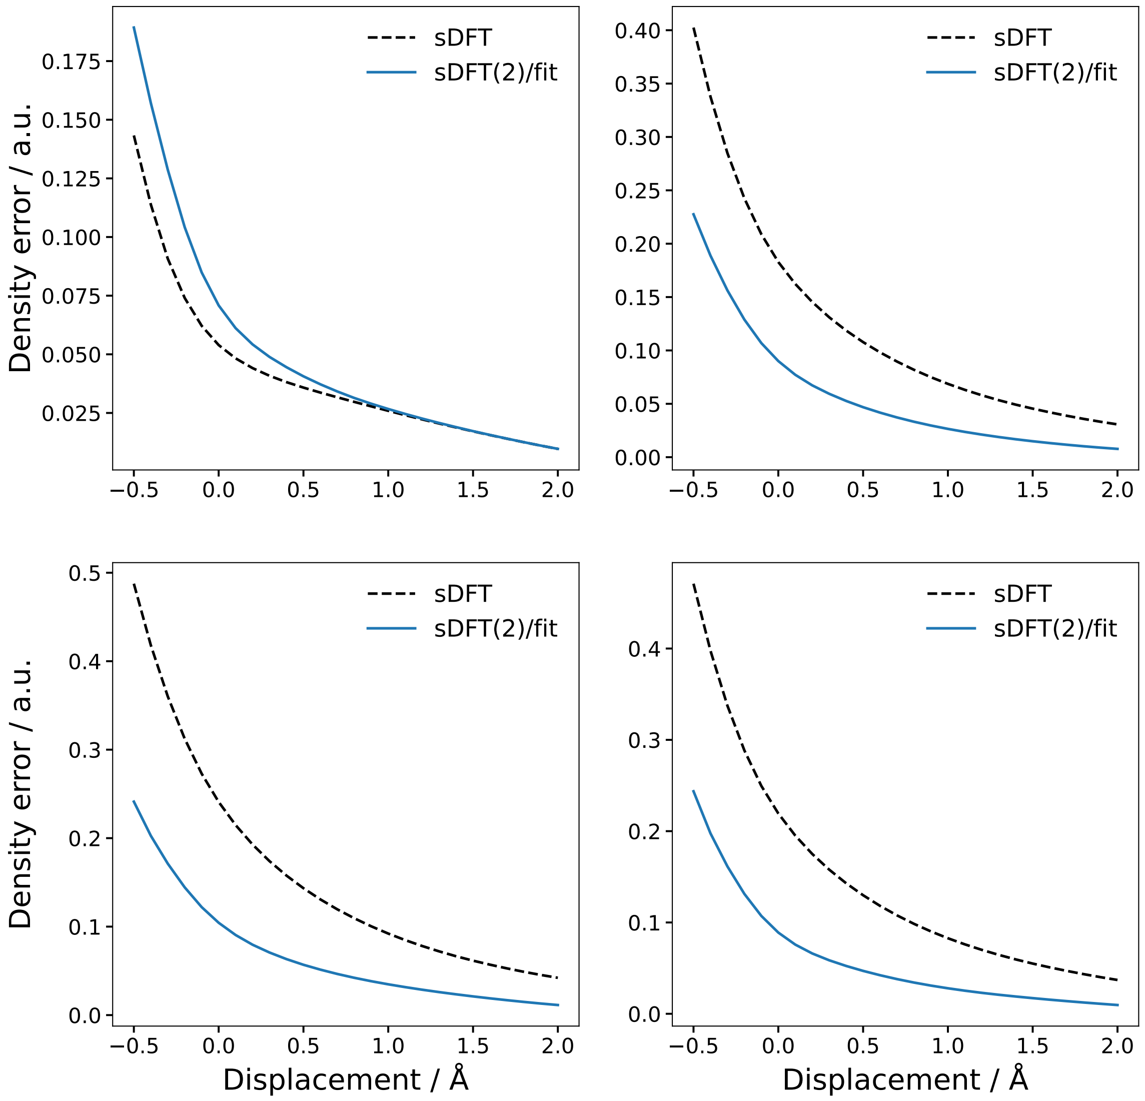


Figure S5: Integrated density errors as functions of the intermolecular displacement. Results are demonstrated for the $H_2O\cdots H_2O$ (top left), $H_2O\cdots CH_3OH$ (top right), $H_2O\cdots (CH_3)_2O$ (bottom left), and $CH_3OH\cdots CH_3OH$ (bottom right) molecular complexes. KS-DFT, sDFT, and sDFT(2)/fit computations are performed using the PW91 XC functional and def2-TZVP basis set. The PW91k kinetic energy functional is employed in sDFT. KS-DFT electron densities serve as the reference.

# References

[1] C. von Neumann. *Untersuchungen über das logarithmische und Newton'sche Potential.* Leipzig : B. G. Teubner, 1877.

[2] M. Renardy, R. C. Rogers. *An Introduction to Partial Differential Equations.* Springer New York, NY, 2 ed., 2004.

[3] E. Engel, R. M. Dreizler. *Density Functional Theory: An Advanced Course.* Springer-Verlag: Berlin, 2011.

[4] R. Courant, D. Hilbert. *Methods of Mathematical Physics.* John Wiley & Sons, Ltd, 1989.

[5] N. J. Higham. *Functions of Matrices – Theory and Computation.* Society for Industrial and Applied Mathematics, Philadelphia, 2008.
